# Supplementary material for: A Domain-Specific Language for Programming in the Tile Assembly Model
Source: arXiv:0903.0889 source file (2009-03-05)
Supplement: Supplementary file 1 [file appendix.tex]

\section{Appendix}
\label{sec-appendix}

\subsection{Notation and Definitions}
\preliminaries
